# Supplementary material for: Many-body correlations brought to light in absorption spectra of diluted magnetic semiconductors
Source: arXiv:1807.04490 ancillary file (2018-10-02)
Supplement: Supplementary file 1 [file paper_supplement.pdf]

# Supplement: Extracting many-body correlation energies from absorption spectra of diluted magnetic semiconductors

F. Ungar,[1] M. Cygorek,[2] and V. M. Axt[1]

[1] *Theoretische Physik III, Universität Bayreuth, 95440 Bayreuth, Germany*

[2] *Department of Physics, University of Ottawa, Ottawa, Ontario, Canada K1N 6N5*

## HAMILTONIAN

The Hamiltonian for the description of the excitation and the dynamics of a II-VI DMS quantum well in the electron-hole representation reads [1, 2]

$$H = H_0 + H_{\text{conf}} + H_{\text{C}} + H_{\text{lm}} + H_{\text{m}} + H_{\text{nm}} + H_{\text{ph}} + H_{\text{c-ph}}, \tag{1}$$

where $H_0$ contains the kinetic energies of electrons and holes in the effective mass approximation, $H_{\text{conf}}$ describes the confinement in the growth direction, and $H_{\text{C}}$ comprises the direct Coulomb interactions that can be subdivided into electron-hole, electron-electron, and hole-hole interactions. The light-matter coupling is given by $H_{\text{lm}}$, whereas $H_{\text{m}}$ and $H_{\text{nm}}$ refer to the magnetic and nonmagnetic carrier-impurity interaction, respectively. Here, we extend the previously developed model [1] to also account for phonons via $H_{\text{ph}}$ and the carrier-phonon interaction $H_{\text{c-ph}}$. The individual contributions are given by

$$H_0 = \sum_{l\mathbf{k}} E^l_{\mathbf{k}} c^\dagger_{l\mathbf{k}} c_{l\mathbf{k}} + \sum_{v\mathbf{k}} E^v_{\mathbf{k}} d^\dagger_{v\mathbf{k}} d_{v\mathbf{k}}, \tag{2a}$$

$$H_{\text{C}} = \frac{1}{2} \sum_{\mathbf{k}\mathbf{k}'\mathbf{q}} \Big( V_{\mathbf{q}} \sum_{ll'} c^\dagger_{l'\mathbf{k}'+\mathbf{q}} c^\dagger_{l\mathbf{k}-\mathbf{q}} c_{l\mathbf{k}} c_{l'\mathbf{k}'} + V_{\mathbf{q}} \sum_{vv'} d^\dagger_{v'\mathbf{k}'+\mathbf{q}} d^\dagger_{v\mathbf{k}-\mathbf{q}} d_{v\mathbf{k}} d_{v'\mathbf{k}'} - 2V_{\mathbf{q}} \sum_{lv} c^\dagger_{l\mathbf{k}'+\mathbf{q}} d^\dagger_{v\mathbf{k}-\mathbf{q}} d_{v\mathbf{k}} c_{l\mathbf{k}'} \Big), \tag{2b}$$

$$H_{\text{lm}} = -\sum_{lv\mathbf{k}} \Big( \mathbf{E}\cdot\mathbf{M}_{lv} c^\dagger_{l\mathbf{k}} d^\dagger_{v-\mathbf{k}} + \mathbf{E}\cdot\mathbf{M}_{vl} d_{v-\mathbf{k}} c_{l\mathbf{k}} \Big), \tag{2c}$$

$$H_{\text{m}} = H_{sd} + H_{pd} = \frac{J_{sd}}{V} \sum_{\substack{Inn'\\ ll'\mathbf{k}\mathbf{k}'}} \mathbf{S}_{nn'} \cdot \mathbf{s}^{\text{e}}_{ll'} c^\dagger_{l\mathbf{k}} c_{l'\mathbf{k}'} e^{i(\mathbf{k}'-\mathbf{k})\cdot\mathbf{R}_I} \hat{P}^I_{nn'} + \frac{J_{pd}}{V} \sum_{\substack{Inn'\\ vv'\mathbf{k}\mathbf{k}'}} \mathbf{S}_{nn'} \cdot \mathbf{s}^{\text{h}}_{vv'} d^\dagger_{v\mathbf{k}} d_{v'\mathbf{k}'} e^{i(\mathbf{k}'-\mathbf{k})\cdot\mathbf{R}_I} \hat{P}^I_{nn'}, \tag{2d}$$

$$H_{\text{nm}} = H^{\text{e}}_{\text{nm}} + H^{\text{h}}_{\text{nm}} = \frac{J^{\text{e}}_0}{V} \sum_{\substack{Il\\ \mathbf{k}\mathbf{k}'}} c^\dagger_{l\mathbf{k}} c_{l\mathbf{k}'} e^{i(\mathbf{k}'-\mathbf{k})\cdot\mathbf{R}_I} + \frac{J^{\text{h}}_0}{V} \sum_{\substack{Iv\\ \mathbf{k}\mathbf{k}'}} d^\dagger_{v\mathbf{k}} d_{v\mathbf{k}'} e^{i(\mathbf{k}'-\mathbf{k})\cdot\mathbf{R}_I}, \tag{2e}$$

$$H_{\text{ph}} = \sum_{\mathbf{q}} \hbar\omega^{\text{ph}}_{\mathbf{q}} b^\dagger_{\mathbf{q}} b_{\mathbf{q}}, \tag{2f}$$

$$H_{\text{c-ph}} = \sum_{\mathbf{q}\mathbf{k}} \Big( \gamma^{\text{e}}_{\mathbf{q}} c^\dagger_{\mathbf{k}+\mathbf{q}} c_{\mathbf{k}} b_{\mathbf{q}} + \gamma^{\text{e}\,*}_{\mathbf{q}} c^\dagger_{\mathbf{k}} c_{\mathbf{k}+\mathbf{q}} b^\dagger_{\mathbf{q}} + \gamma^{\text{h}}_{\mathbf{q}} d^\dagger_{\mathbf{k}+\mathbf{q}} d_{\mathbf{k}} b_{\mathbf{q}} + \gamma^{\text{h}\,*}_{\mathbf{q}} d^\dagger_{\mathbf{k}} d_{\mathbf{k}+\mathbf{q}} b^\dagger_{\mathbf{q}} \Big). \tag{2g}$$

In the above equations, $c^\dagger_{l\mathbf{k}}$ ($c_{l\mathbf{k}}$) denotes the electron creation (annihilation) operator in the conduction band $l$ with wave vector $\mathbf{k}$ and $d^\dagger_{v\mathbf{k}}$ ($d_{v\mathbf{k}}$) is the respective creation (annihilation) operator for holes in the valence band $v$. The Fourier components of the bulk Coulomb potential are given by $V_{\mathbf{q}} = \frac{e^2}{\epsilon\epsilon_0}\frac{1}{q^2}$ with the elementary charge $e$, the vacuum permittivity $\epsilon_0$, and a static dielectric constant $\epsilon$. In the light-matter interaction, $\mathbf{E}$ denotes the electric field and $\mathbf{M}_{lv}$ is the dipole moment for a transition from the valence subband $v$ to the conduction subband $l$. We denote the vector of electron spin matrices by $\mathbf{s}^{\text{e}}_{ll'} = \frac{1}{2}\boldsymbol{\sigma}_{ll'}$, where $\boldsymbol{\sigma}_{ll'}$ is the vector of Pauli matrices, and $\mathbf{s}^{\text{h}}_{vv'} = \frac{1}{3}\mathbf{J}_{vv'}$ describes the hole spin in terms of the vector of $4\times4$ angular momentum matrices $\mathbf{J}_{vv'}$ with $v, v' \in \{-\frac{3}{2}, -\frac{1}{2}, \frac{1}{2}, \frac{3}{2}\}$. In the magnetic interaction, $\mathbf{S}_{nn'}$ denotes the vector of impurity spin matrices with $n, n' \in \{-\frac{5}{2}, -\frac{3}{2}, ..., \frac{5}{2}\}$. To describe the impurity spin at a particular site in the DMS, we make use of the operator $\hat{P}^I_{nn'} = |I, n\rangle\langle I, n'|$ where the ket $|I, n\rangle$ denotes the spin state $n$ of the $I$th impurity atom and $\mathbf{R}_I$ refers to its position. Throughout this paper, the factor $\hbar$ appearing in the spin matrices is absorbed in the coupling constants $J_{sd}$ and $J_{pd}$. Finally, $J^{\text{e}}_0$ and $J^{\text{h}}_0$ are nonmagnetic scattering constants for electrons and holes that arise due to the band-gap mismatch of the doped material compared with the undoped barriers of the quantum well. The creation (annihilation) operators for acoustic phonons with wave vector $\mathbf{q}$ are denoted by $b^\dagger_{\mathbf{q}}$ ($b_{\mathbf{q}}$) with frequencies $\omega^{\text{ph}}_{\mathbf{q}} = vq$, where $v$ is the sound velocity and a linear dispersion is assumed.

The deformation potential coupling for electrons and holes is given by $\gamma_{\mathbf{q}}^{\mathrm{e/h}} = \sqrt{\frac{\hbar q}{2\rho v V}} D^{\mathrm{e/h}}$ with the density $\rho$ of the semiconductor and the deformation potentials $D^{\mathrm{e/h}}$.

## EQUATIONS OF MOTION FOR THE COHERENCE AND ITS CORRELATIONS

In the exciton representation, the necessary variables to describe the linear absorption for an excitation with circularly polarized ($\sigma^-$) light in the absence of an external magnetic field are [1, 2]

$$y := \left\langle \hat{Y}_{\uparrow-\frac{3}{2}1s0} \right\rangle, \tag{3a}$$

$$q_{\eta K} := \frac{Vd}{N_{\mathrm{Mn}}} \int_0^{2\pi} \frac{d\psi}{2\pi} f_{\eta 1s1s}^{0\mathbf{K}} \int_{-\frac{d}{2}}^{\frac{d}{2}} dz\, |u_0(z)|^2 \sum_{Inn'} S_{nn'}^z \left\langle \hat{Y}_{\uparrow-\frac{3}{2}1s\mathbf{K}} e^{i\mathbf{K}\cdot\mathbf{R}_I} \hat{P}_{nn'}^I \delta(z-Z_I) \right\rangle, \tag{3b}$$

$$z_{\eta K} := \frac{Vd}{N_{\mathrm{Mn}}} \int_0^{2\pi} \frac{d\psi}{2\pi} f_{\eta 1s1s}^{0\mathbf{K}} \int_{-\frac{d}{2}}^{\frac{d}{2}} dz\, |u_0(z)|^2 \sum_{I} \left\langle \hat{Y}_{\uparrow-\frac{3}{2}1s\mathbf{K}} e^{i\mathbf{K}\cdot\mathbf{R}_I} \delta(z-Z_I) \right\rangle, \tag{3c}$$

$$p_K^\kappa := \int_0^{2\pi} \frac{d\psi_1}{2\pi} f(\kappa) \big( \gamma_{\mathbf{K},\kappa}^{\mathrm{e}} f_{-\eta_{\mathrm{h}}1s1s}^{\mathbf{K}\mathbf{0}} + \gamma_{\mathbf{K},\kappa}^{\mathrm{h}} f_{\eta_{\mathrm{e}}1s1s}^{\mathbf{K}\mathbf{0}} \big) \langle \hat{Y}_{\uparrow-\frac{3}{2}1s\mathbf{K}} b_{\mathbf{K},\kappa} \rangle, \tag{3d}$$

$$\tilde{p}_K^\kappa := \int_0^{2\pi} \frac{d\psi_1}{2\pi} f(\kappa)^* \big( \gamma_{\mathbf{K},\kappa}^{\mathrm{e}} f_{-\eta_{\mathrm{h}}1s1s}^{\mathbf{K}\mathbf{0}} + \gamma_{\mathbf{K},\kappa}^{\mathrm{h}} f_{\eta_{\mathrm{e}}1s1s}^{\mathbf{K}\mathbf{0}} \big)^* \langle \hat{Y}_{\uparrow-\frac{3}{2}1s\mathbf{K}} b_{\mathbf{K},\kappa}^\dagger \rangle, \tag{3e}$$

which refer to the electron-hole coherence ($y$) and its correlations due to the magnetic ($q_{\eta K}$) as well as the nonmagnetic ($z_{\eta K}$) interaction with impurities, respectively. Additionally, we have introduced the phonon-assisted variables $p_K^\kappa$ and $\tilde{p}_K^\kappa$. We consider a quantum well of volume $V$ and width $d$ with $N_{\mathrm{Mn}}$ being the number of impurities. The exciton annihilation operator is denoted by $\hat{Y}_{\uparrow-\frac{3}{2}1s\mathbf{K}}$ for the $1s$ exciton ground state with the two dimensional center-of-mass wave vector $\mathbf{K}$ for an electron with spin up ($\uparrow$) and a heavy hole with quantum number $m_J = -\frac{3}{2}$. Note that the optical excitation only couples to the state with $K = 0$ in the dipole approximation. The $z$ direction is chosen to coincide with the growth direction of the quantum well and $u_0(z)$ denotes the envelope function due to the confinement, for which we consider only the energetically lowest state since we are dealing with sufficiently narrow quantum wells. In addition, the expectation value $\langle . \rangle$ contains an average over the distribution of impurity positions, which are assumed to be random but spatially homogeneous on average in the sample. Finally, the variables are averaged over the angle $\psi$ with respect to the center-of-mass wave vector $\mathbf{K}$ and the appearing form factors for the exciton ground state read [2]

$$f_{\eta 1s1s}^{\mathbf{K}_1\mathbf{K}_2} = 2\pi \int_0^\infty dr\, R_{1s}^2(r) J_0\big(\eta |\mathbf{K}_1 - \mathbf{K}_2| r\big), \tag{4}$$

where the constants $\eta_{\mathrm{e}} = m_{\mathrm{e}}/M$ as well as $\eta_{\mathrm{h}} = m_{\mathrm{h}}/M$ denote the ratio between the effective electron or heavy-hole mass and the exciton mass $M = m_{\mathrm{e}} + m_{\mathrm{h}}$, respectively. Furthermore, $\eta \in \{\eta_{\mathrm{e}}, \eta_{\mathrm{h}}\}$ and the function $J_0(x)$ is the cylindrical Bessel function of order zero. Regarding the phonon-assisted variables, the phonon wave vector is split into an in-plane component $\mathbf{K}$ and a one dimensional component $\kappa$ so that the total phonon wave number which enters the carrier-phonon coupling is given by $\sqrt{\mathbf{K}^2 + \kappa^2}$. Projecting the phonon dynamics onto the confinement ground state then yields the phonon form factor

$$f(\kappa) = \sum_z u_0^{\mathrm{e}}(z) u_0^{\mathrm{h}}(z) e^{i\kappa z} = \frac{\sin\left(\frac{\kappa d}{2}\right)}{\frac{\kappa d}{2}} \left[ 1 - \left( \frac{\kappa d}{2\pi} \right)^2 \right]^{-1}.$$

Extending the equations of motion derived in Ref. [1] by also accounting for the phonon influence, the coupled equations for the coherence $y$ and its correlation contributions $q_{\eta K}$ and $z_{\eta K}$ in the exciton representation become

$$\frac{\partial}{\partial t} y = \frac{i}{\hbar} \mathbf{E} \cdot \mathbf{M} \phi_{1s} - \Gamma_0(0) y - i \frac{N_{\mathrm{Mn}}}{2\hbar V^2} \int_0^{K_{\mathrm{c}}} dK\, D(K) \big( J_{sd} q_{-\eta_{\mathrm{h}}K} - J_{pd} q_{\eta_{\mathrm{e}}K} + 2 J_0^{\mathrm{e}} z_{-\eta_{\mathrm{h}}K} + 2 J_0^{\mathrm{h}} z_{\eta_{\mathrm{e}}K} \big)$$
$$- i \frac{d}{\pi\hbar} \int_0^{K_{\mathrm{c}}} dK\, D(K) \int_0^{K_{\mathrm{c}}} d\kappa\, \big( p_K^\kappa + \tilde{p}_K^\kappa \big), \tag{5a}$$

$$\frac{\partial}{\partial t} q_{\eta K} = -\big(i\omega_K + \Gamma_0(K)\big) q_{\eta K} - i\frac{35 I}{24\hbar}\Big(J_{sd} F^{-\eta_{\rm h} 0 K}_{\eta\ 1s1s} - J_{pd} F^{\eta_{\rm e} 0 K}_{\eta\ 1s1s}\Big) y, \tag{5b}$$

$$\frac{\partial}{\partial t} z_{\eta K} = -\big(i\omega_K + \Gamma_0(K)\big) z_{\eta K} - i\frac{I}{\hbar}\Big(J_0^{\rm e} F^{-\eta_{\rm h} 0 K}_{\eta\ 1s1s} + J_0^{\rm h} F^{\eta_{\rm e} 0 K}_{\eta\ 1s1s}\Big) y, \tag{5c}$$

$$\frac{\partial}{\partial t} p_K^{\kappa} = -i\big(\omega_K + \omega^{\rm ph}_{K,\kappa} + \Gamma_0(K)\big) p_K^{\kappa} - i\frac{\sqrt{K^2+\kappa^2}}{2\rho v V}|f(\kappa)|^2\Big(D_{\rm e}^2 F^{\eta_{\rm h} 0 K}_{\eta_{\rm h} 1s1s} + D_{\rm h}^2 F^{\eta_{\rm e} 0 K}_{\eta_{\rm e} 1s1s} + 2D_{\rm e}D_{\rm h} F^{\ \eta_{\rm e} 0 K}_{-\eta_{\rm h} 1s1s}\Big)(1+n^{\rm ph}_{K,\kappa}) y, \tag{5d}$$

$$\frac{\partial}{\partial t} \tilde{p}_K^{\kappa} = -i\big(\omega_K - \omega^{\rm ph}_{K,\kappa} + \Gamma_0(K)\big) \tilde{p}_K^{\kappa} - i\frac{\sqrt{K^2+\kappa^2}}{2\rho v V}|f(\kappa)|^2\Big(D_{\rm e}^2 F^{\eta_{\rm h} 0 K}_{\eta_{\rm h} 1s1s} + D_{\rm h}^2 F^{\eta_{\rm e} 0 K}_{\eta_{\rm e} 1s1s} + 2D_{\rm e}D_{\rm h} F^{\ \eta_{\rm e} 0 K}_{-\eta_{\rm h} 1s1s}\Big) n^{\rm ph}_{K,\kappa} y. \tag{5e}$$

The first term in Eq. (5a) describes the driving by the laser field where $\phi_{1s} = R_{1s}(r=0)$ is the radial part of the $1s$ exciton wave function evaluated at $r=0$. Radiative decay is included in the equations via the $K$ dependent rate $\Gamma_0(K) = \Gamma_0\Theta(E_{1s} + \hbar\omega_K - \hbar c K)$ derived from the condition of energy conservation upon photon emission [3, 4]. In practice, this means that only excitons close to $K=0$ are affected by radiative decay. The third term captures the influence of magnetic and nonmagnetic exciton-impurity correlations and the double integral finally accounts for the phonon influence. The equations are formulated in the rotating frame with respect to the $1s$ exciton frequency and we have made use of the rotating-wave approximation so that $\mathbf{E}$ contains only the slowly varying envelope of the laser. In the effective-mass approximation, the exciton dispersion reads $\omega_K = \hbar K^2/2M$. Furthermore, we have used the continuum limit for the center-of-mass wave number $K$ with the density of states given by $D(K) = AK/2\pi$. The cutoff value $K_{\rm c}$ appearing in the integral over the correlations is chosen such that it corresponds to an energy of 100 meV. This should be compared with the exciton binding energy which, for a 10 nm wide ZnSe quantum well, is approximately 30 meV. Thus, it is ensured that all oscillating terms encountered in Eqs. (5) are numerically well resolved. In the equations for the correlations, the factor $I = 3/2$ stems from the projection of all quantities onto the lowest confinement state in the growth direction, for which the approximation of an infinitely deep quantum well is employed. Finally, the angle-averaged exciton form factors are given by

$$F^{\eta_2 K_1 K_2}_{\eta_1 1s1s} = 2\pi\int_0^{2\pi} d\psi_{12}\int_0^{\infty} dr\int_0^{\infty} dr'\, rr' R_{1s}^2(r) R_{1s}^2(r') J_0\big(\eta_1 K_{12}(\psi_{12}) r\big) J_0\big(\eta_2 K_{12}(\psi_{12}) r'\big), \tag{6}$$

where $K_{12} = |\mathbf{K}_1 - \mathbf{K}_2|$ with $\psi_{12}$ describing the angle between $\mathbf{K}_1$ and $\mathbf{K}_2$. It should be noted that, in order to arrive at Eq. (5d) and Eq. (5e), we have assumed the phonons to be in thermal equilibrium with an occupation given by $n^{\rm ph}_{K,\kappa} = 1/(\exp(\hbar v\sqrt{K^2+\kappa^2}/k_B T) - 1)$.

## LINEAR RESPONSE

The linear response can be obtained from Eqs. (5) by formally integrating Eqs. (5b)–(5e) and feeding the results back into Eq. (5a), which yields an integro-differential equation for the coherence $y(t)$. Applying the Fourier transform in the time domain and making use of the convolution theorem then allows one to transform Eq. (5a) into an algebraic equation that can be solved for the coherence $y(\omega)$. The relation between the coherence and the polarization subsequently yields the complex susceptibility

$$\chi(\omega) \sim \frac{-1}{\omega + i\Gamma_0(0) + \int_0^{K_{\rm c}} dK \frac{D(K)\Gamma^2_{\rm imp}(K)}{\omega_K - \omega - i\Gamma_0(K)} + \int_0^{K_{\rm c}} dK \int_0^{K_{\rm c}} d\kappa\, \frac{D(K)\Gamma^2_{\rm ph}(K,\kappa) d}{\pi}\left(\frac{1+n^{\rm ph}_{K,\kappa}}{\omega_K + \omega^{\rm ph}_{K,\kappa} - \omega - i\Gamma_0(K)} + \frac{n^{\rm ph}_{K,\kappa}}{\omega_K - \omega^{\rm ph}_{K,\kappa} - \omega - i\Gamma_0(K)}\right)} \tag{7}$$

with

$$\Gamma^2_{\rm imp}(K) = \frac{I N_{\rm Mn}}{\hbar^2 V^2}\left(\left(\frac{35}{48}J_{sd}^2 + J_0^{\rm e\,2}\right) F^{\eta_{\rm h} 0 K}_{\eta_{\rm h} 1s1s} + \left(2J_0^{\rm e} J_0^{\rm h} - \frac{35}{24}J_{sd}J_{pd}\right) F^{\ \eta_{\rm e} 0 K}_{-\eta_{\rm h} 1s1s} + \left(\frac{35}{48}J_{pd}^2 + J_0^{\rm h\,2}\right) F^{\eta_{\rm e} 0 K}_{\eta_{\rm e} 1s1s}\right), \tag{8}$$

$$\Gamma^2_{\rm ph}(K,\kappa) = \frac{\sqrt{K^2+\kappa^2}}{2\hbar\rho v V}|f(\kappa)|^2\Big(D_{\rm e}^2 F^{\eta_{\rm h} 0 K}_{\eta_{\rm h} 1s1s} + D_{\rm h}^2 F^{\eta_{\rm e} 0 K}_{\eta_{\rm e} 1s1s} + 2D_{\rm e}D_{\rm h} F^{\ \eta_{\rm e} 0 K}_{-\eta_{\rm h} 1s1s}\Big). \tag{9}$$

The linear absorption is given by the imaginary part of $\chi$.

Neglecting the phonon influence and separating $\chi$ into its real and imaginary part, one arrives at

$$\chi \sim -\frac{\omega + {\rm Re}[\Sigma(\omega)]}{\big(\omega + {\rm Re}[\Sigma(\omega)]\big)^2 + \big(\Gamma_0(K) + {\rm Im}[\Sigma(\omega)]\big)^2} + i\frac{\Gamma_0(K) + {\rm Im}[\Sigma(\omega)]}{\big(\omega + {\rm Re}[\Sigma(\omega)]\big)^2 + \big(\Gamma_0(K) + {\rm Im}[\Sigma(\omega)]\big)^2} \tag{10}$$

with a complex self energy resulting from the interaction between carriers and magnetic impurities given by

$$\hbar\Sigma(\omega) = \int_0^{K_c} dK\, D(K) \frac{\hbar(\omega_K - \omega)\Gamma_{\rm imp}^2(K)}{(\omega_K - \omega)^2 + \Gamma_0(K)^2} + i \int_0^{K_c} dK\, D(K) \frac{\hbar\Gamma_0(K)\Gamma_{\rm imp}^2(K)}{(\omega_K - \omega)^2 + \Gamma_0(K)^2}. \tag{11}$$

It is straightforward to show that $\mathrm{Im}[\Sigma(\omega)] \geq 0\,\forall\,\omega$ and, as a consequence, $\mathrm{Im}[\chi] \geq 0\,\forall\,\omega$. We model the radiative decay by

$$\Gamma_0(K) = (\Gamma_0 - \gamma)\exp\left(-\left(\frac{\hbar\omega_K}{2w}\right)^2\right) + \gamma \tag{12}$$

which satisfies $\Gamma_0(0) = \Gamma_0$. The width of the Gaussian is chosen to be $w = 1\,\mu$eV so that only states in close proximity to $K = 0$ undergo radiative decay. Furthermore, we have introduced the constant $\gamma \ll \Gamma_0$ that enables a faster convergence of the numerical result. It has been carefully checked and verified that the numerical values for the linear absorption obtained from Eq. (7) coincide with the full solution of Eqs. (5) in the time domain and subsequent Fourier transform.

## AVERAGE CORRELATION ENERGY PER EXCITON

The correlation energy due to the magnetic and nonmagnetic exciton-impurity interactions is obtained by subtracting the mean-field contribution from the expectation value of the respective parts of the Hamiltonian given by Eq. (1). Following Ref. 2, the correlation energies can be written as

$$\langle H_{\rm m}\rangle^{\rm c} = \frac{N_{\rm Mn}}{V^2}\int_0^{K_c} dK \int_0^{K_c} dK'\, D(K)D(K')\Big(J_{sd}\sum_l Q_{-\eta_{\rm h}lK}^{\;\;lK'}(t) - \frac{J_{pd}}{2}Q_{\eta_{\rm e}zK}^{\;\;0K'}\Big), \tag{13a}$$

$$\langle H_{\rm nm}\rangle^{\rm c} = \frac{N_{\rm Mn}}{V^2}\int_0^{K_c} dK \int_0^{K_c} dK'\, D(K)D(K')\Big(J_0^{\rm e} Z_{-\eta_{\rm h}\;K}^{\;\;0K'}(t) + J_0^{\rm h} Z_{\eta_{\rm e}\;K}^{\;\;0K'}\Big), \tag{13b}$$

with the correlations

$$Q_{\eta l K_1}^{\;\alpha K_2} = \frac{Vd}{N_{\rm Mn}}\int_0^{2\pi}\frac{d\psi_1}{2\pi}\int_0^{2\pi}\frac{d\psi_2}{2\pi} f_{\eta 1s1s}^{\mathbf{K}_1\mathbf{K}_2}\int dz|u_0(z)|^2 \sum_{\substack{\sigma\sigma' I\\ nn'}} S_{nn'}^l s_{\sigma\sigma'}^{\rm e,\alpha}\Big\langle \hat{Y}^\dagger_{\sigma-\frac{3}{2}1s\mathbf{K}_1}\hat{Y}_{\sigma'-\frac{3}{2}1s\mathbf{K}_2} e^{i(\mathbf{K}_2-\mathbf{K}_1)\cdot\mathbf{R}_I}\hat{P}^I_{nn'}\delta(z-Z_I)\Big\rangle, \tag{14a}$$

$$Z_{\eta\;K_1}^{\;\alpha K_2} = \frac{Vd}{N_{\rm Mn}}\int_0^{2\pi}\frac{d\psi_1}{2\pi}\int_0^{2\pi}\frac{d\psi_2}{2\pi} f_{\eta 1s1s}^{\mathbf{K}_1\mathbf{K}_2}\int dz|u_0(z)|^2 \sum_{\sigma\sigma' I} s_{\sigma\sigma'}^{\rm e,\alpha}\Big\langle \hat{Y}^\dagger_{\sigma-\frac{3}{2}1s\mathbf{K}_1}\hat{Y}_{\sigma'-\frac{3}{2}1s\mathbf{K}_2} e^{i(\mathbf{K}_2-\mathbf{K}_1)\cdot\mathbf{R}_I}\delta(z-Z_I)\Big\rangle. \tag{14b}$$

The correlation energy is obtained by solving the equations of motion for these correlations, which are given explicitly in Ref. 2. An analysis of the prefactors in Eqs. (13) and Eqs. (14) together with the scaling of the density of states yields an inverse dependence of the total correlation energy $\langle H_{\rm m} + H_{\rm nm}\rangle^{\rm c}$ on the quantum well width. Since the so defined correlation energy depends on the strength of the optical excitation and thus on the number of excited excitons, it is preferable to instead consider the correlation energy per exciton as this quantity is independent on the optical driving strength in the low-intensity regime. However, due to the optical excitation as well as radiative decay, the correlation energy is a time-dependent quantity. A reliable value for the average correlation energy per exciton is then given by

$$\overline{E_{\rm corr}} = \frac{1}{T}\int_0^T dt\, E_{\rm corr}(t) = \frac{1}{T}\int_0^T dt\, \frac{\langle H_{\rm m} + H_{\rm nm}\rangle^{\rm c}(t)}{n_{\rm X}(t)}, \tag{15}$$

where $n_{\rm X}(t)$ denotes the number of excitons at time $t$ and $T$ is a suitably long averaging time.

In order to provide an example for the time dependence of the correlation energy as well as the extraction of its corresponding average per exciton, Fig. 1 shows the correlation energy calculated using Eqs. (13) for a 15 nm wide $Zn_{0.975}Mn_{0.025}Se$ quantum well with acoustic phonon scattering at 30 K and a radiative decay rate of $0.1\,\mathrm{ps}^{-1}$. Looking first at the number of excitons in Fig. 1(a) and the correlation energy in Fig. 1(b), the influence of radiative decay causes both quantities to decrease over time after the pulse is switched off. Note that this decrease occurs on large time scales compared to the radiative decay rate since only excitons close to $K = 0$ are allowed to recombine.

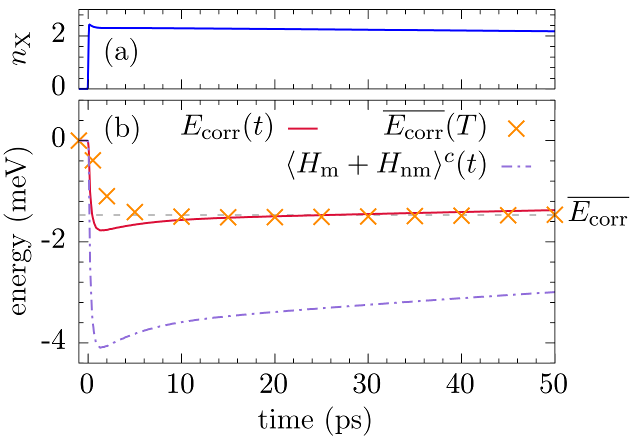


FIG. 1. Build up of the correlation energy in a 15 nm wide $Zn_{0.975}Mn_{0.025}Se$ quantum well at 30 K. We compare (a) the number of excitons $n_X$ with (b) the correlation energy given by the expectation value $\langle H_m + H_{nm}\rangle^c(t)$. Also shown is the time-dependent quotient $E_{corr}(t)$ from Eq. (15) in relation to the time-averaged correlation energy per exciton $\overline{E_{corr}}(T)$ as a function of the averaging time. The final value for the average correlation energy per exciton is marked by $\overline{E_{corr}}$ and the grey dashed line. For the optical excitation, a 100 fs laser pulse is assumed.

Due to the pronounced scattering of excitons at the impurities as well as the scattering due to phonons, optically created excitons are scattered away from $K = 0$ and are thus no longer affected by radiative decay, which effectively slows down the decay.

Figure 1(b) also shows the time dependent correlation energy per exciton $E_{corr}(t)$ obtained from the quotient of the correlation energy and the number of excitons. Since both numerator and denominator in this quotient are decreasing as a function of time, the resulting quantity is much less affected by radiative decay and shows almost no time dependence after an initial overshoot that can be attributed to the energy-time uncertainty regarding the optical excitation. Fig. 1(b) confirms that $\overline{E_{corr}}(T)$ then indeed yields a reliable number for the correlation energy per exciton that remains virtually constant after an averaging time of about 10 ps. The final value of the average correlation energy per exciton used for the interpretation of the linear absorption spectra is marked by $\overline{E_{corr}}$.


[1] F. Ungar, M. Cygorek, and V. M. Axt, Phys. Rev. B **95**, 245203 (2017).
[2] F. Ungar, M. Cygorek, and V. M. Axt, Phys. Rev. B **97**, 045210 (2018).
[3] A. Thränhardt, S. Kuckenburg, A. Knorr, T. Meier, and S. W. Koch, Phys. Rev. B **62**, 2706 (2000).
[4] K. Siantidis, V. M. Axt, and T. Kuhn, Phys. Rev. B **65**, 035303 (2001).
